# Supplementary material for: Mini-Batch Optimization of Contrastive Loss
Source: arXiv:2307.05906 source file (2023-07-12)
Supplement: Supplementary file 1 [file FigAppendix.tex]

\begin{figure}[!h]
\centering
\includegraphics[width=0.98\columnwidth]{neurips2023/figures/exps/exp1_blue.png}
\vspace{-3mm}
\caption{Histograms of contrastive loss for randomly shuffled batches across multiple epochs (epoch=0, 1, 51, 101). As the training progresses, the loss is decreasing and the histogram is skewed to the left. \\ Dataset: CIFAR-10, Model: ResNet-50, Batch Sample Algorithm: OSGD\_kb, Epoch: \{0, 1, 51, 101\}, N: 50,000, B: 20, N//B: 2,500, raw data: N//B batches' contrastive loss.}
\label{fig:concept}
\end{figure}

\begin{figure}[!h]
\centering
\includegraphics[width=0.98\columnwidth]{neurips2023/figures/exps/exp1_green.png}
\vspace{-3mm}
\caption{Histograms of contrastive loss for randomly shuffled batches across multiple epochs (epoch=0, 1, 51, 101). As the training progresses, the loss is decreasing and the histogram is skewed to the left. \\ Dataset: CIFAR-10, Model: ResNet-50, Batch Sample Algorithm: OSGD\_kb, Epoch: \{0, 1, 51, 101\}, N: 50,000, B: 20, N//B: 2,500, raw data: N//B batches' contrastive loss.}
\label{fig:concept}
\end{figure}

\begin{figure}[!h]
\centering
\includegraphics[width=0.98\columnwidth]{neurips2023/figures/exps/exp2_colored.png}
\vspace{-3mm}
\caption{Histograms of contrastive loss for random shuffled batches across multiple epochs (row-wise) and various batch size (column-wise). As the training progresses, the loss is decreasing and the histogram is skewed to the left (except B= 100). \\ Dataset: CIFAR-10, Model: ResNet-50, Batch Sample Algorithm: OSGD\_kb, Epoch: \{0, 1, 51, 101\}, N: 50,000, B: \{20, 100, 1,000, 2,500\}, raw data: N//B batches' contrastive loss.}
\label{fig:concept}
\end{figure}

\begin{figure}[!h]
\centering
\includegraphics[width=0.98\columnwidth]{neurips2023/figures/exps/exp2_uncolored.png}
\vspace{-3mm}
\caption{Histograms of contrastive loss for random shuffled batches across multiple epochs (row-wise) and various batch size (column-wise). As the training progresses, the loss is decreasing and the histogram is skewed to the left (except B= 100). \\ Dataset: CIFAR-10, Model: ResNet-50, Batch Sample Algorithm: OSGD\_kb, Epoch: \{0, 1, 51, 101\}, N: 50,000, B: \{20, 100, 1,000, 2,500\}, raw data: N//B batches' contrastive loss.}
\label{fig:concept}
\end{figure}

\begin{figure}[!h]
\centering
\includegraphics[width=0.98\columnwidth]{neurips2023/figures/exps/true_loss.png}
\vspace{-3mm}
\caption{True loss plot. the iterative algorithm's true loss is the lowest, even if the gap is marginal. \\ Pre-trained Dataset: CIFAR-100, Model: ResNet-50, N: 50,000, B: 20}
\label{fig:concept}
\end{figure}

\begin{figure}[!h]
\centering
\includegraphics[width=0.98\columnwidth]{neurips2023/figures/exps/linear_eval.png}
\vspace{-3mm}
\caption{Comparison of linear classification performance for batch selection algorithms 
 on image datasets (1. ImageNet-a \& subset of ImageNet, 2. CIFAR100)}
\label{fig:concept}
\end{figure}

\begin{figure}[!h]
\centering
\includegraphics[width=0.48\columnwidth]{neurips2023/figures/exps/random_batch_hist.png}
\vspace{-3mm}
\caption{Histogram of contrastive loss of random batches utilizing models trained with various batch selection algorithms (random, osgd\_kb (max), spectral clustering). Each model is train at 101 epoches.}
\label{fig:concept}
\end{figure}

\begin{figure}[!h]
\centering
\includegraphics[width=0.98\columnwidth]{neurips2023/figures/exps/top1_accu_retrieval.png}
\vspace{-3mm}
\caption{Comparison of top-1 accuracy (Retrieval) of CIFAR100-pretrained ResNet50 models with various batch selection algorithms. Spectral Clustering significantly outperformed the other methods in terms of top-1 accuracy.}
\label{fig:concept}
\end{figure}

\begin{figure}[!h]
\centering
\includegraphics[width=0.98\columnwidth]{neurips2023/figures/exps/cifar100_c.png}
\vspace{-3mm}
\caption{Comparison of linear evaluation performances on the corrupted dataset CIFAR100-c for batch selection algorithms, utilizing CIFAR100-pretrained ResNet50 models. Contrary to our expectations, the spectral clustering algorithm did not perform well in terms of robust accuracy.
Sort of corruption: gaussian blur, brightness, contrast}
\label{fig:concept}
\end{figure}

\begin{figure}[!h]
\centering
\includegraphics[width=0.98\columnwidth]{neurips2023/figures/exps/TinyImageNet_c.png}
\vspace{-3mm}
\caption{Comparison of linear evaluation performances on the corrupted dataset Tiny ImageNet-c for batch selection algorithms, utilizing CIFAR100-pretrained ResNet50 models. Contrary to our expectations, the spectral clustering algorithm did not perform well in terms of robust accuracy.
Sort of corruption: gaussian blur, brightness, contrast}
\label{fig:concept}
\end{figure}

\begin{figure}[!h]
\centering
\includegraphics[width=0.98\columnwidth]{neurips2023/figures/exps/retrieval_corrupted.png}
\vspace{-3mm}
\caption{Top-1 accuracy (retrieval) of various corrupted versions' augmented images retrieval. row: augmentation1(corrupted images from the original image), column: augmentation2(corrupted images from the original image). When performing contrastive learning with high-loss batches, it is possible to make finer distinctions in the embeddings.}
\label{fig:concept}
\end{figure}
